# Supplementary material for: Interpretable Deep Learning for Forecasting Online Advertising Costs: Insights from the Competitive Bidding Landscape
Source: arXiv:2302.05762 source file (2024-08-21)
Supplement: Supplementary file 1 [file appendices.tex]

\begin{sidewaystable}%[!htb]
{ % padding
    \begin{tabular}{p{3cm}p{0.02cm}p{1cm}p{1cm}p{1.2cm}p{0.02cm}p{1cm}p{1cm}p{1.2cm}p{0.02cm}p{1cm}p{1cm}p{1.2cm}}
    \hline
    \textbf{Model} & & & \textbf{14 days} & & & & \textbf{30 days} & & & & \textbf{60 days} & \\
    & & MAE $\downarrow$ & MAPE $\downarrow$ & SMAPE $\downarrow$ & & MAE $\downarrow$ & MAPE $\downarrow$ & SMAPE $\downarrow$ & & MAE $\downarrow$ & MAPE $\downarrow$ & SMAPE $\downarrow$ \\
    \cline{1-1}
    \cline{3-5}
    \cline{7-9}
    \cline{11-13}
        SARIMA.univar & & 0.211 & \textbf{0.184} & 0.179 & & 0.227 & 0.209 & 0.197 & & 0.306 & 0.299 & 0.264 \\
        \vspace{1pt} \\
        XGB.univar & & 0.259 & 0.241 & 0.225 & & 0.278 & 0.262 & 0.243 & & 0.340 & 0.313 & 0.279 \\
        XGB.multivar & & 0.242 & 0.241 & 0.218 & & 0.271 & 0.233 & 0.231 & & 0.274 & 0.282 & 0.258 \\
        XGB.multivar.comp.cat & & 0.245 & 0.227 & 0.219 & & 0.250 & 0.245 & 0.218 & & 0.278 & 0.270 & 0.423 \\
        XGB.multivar.comp.extr & & 0.248 & 0.232 & 0.228 & & 0.257 & 0.242 & 0.216 & & 0.267 & 0.268 & 0.239 \\
        XGB.multivar.comp.dist & & 0.244 & 0.221 & 0.213 & & 0.246 & 0.230 & 0.227 & & 0.276 & 0.263 & 0.235 \\
        \vspace{1pt} \\
        LSTM.univar & & 0.245 & 0.224 & 0.203 & & 0.265 & 0.243 & 0.217 & & 0.318 & 0.287 & 0.251 \\
        LSTM.multivar & & 0.235 & 0.210 & 0.204 & & 0.250 & 0.221 & 0.215 & & 0.252 & 0.253 & 0.236 \\
        LSTM.multivar.comp.cat & & 0.231 & 0.203 & 0.199 & & 0.229 & 0.223 & 0.202 & & 0.253 & 0.233 & 0.228 \\
        LSTM.multivar.comp.extr & & 0.227 & 0.198 & 0.202 & & 0.235 & 0.224 & 0.199 & & 0.253 & 0.244 & 0.237 \\
        LSTM.multivar.comp.dist & & 0.229 & 0.220 & 0.196 & & 0.231 & 0.219 & 0.210 & & 0.250 & 0.236 & 0.232 \\
        \vspace{1pt} \\
        TFT.univar & & 0.216 & 0.197 & 0.185 & & 0.236 & 0.218 & 0.204 & & 0.307 & 0.274 & 0.241 \\
        TFT.multivar & & 0.203 & 0.192 & 0.180 & & 0.223 & 0.203 & 0.192 & & 0.241 & 0.229 & 0.214 \\
        TFT.multivar.comp.cat & & 0.208 & 0.190 & 0.181 & & 0.215 & 0.196 & 0.188 & & 0.238 & 0.223 & 0.204 \\
        TFT.multivar.comp.extr & & 0.207 & 0.191 & 0.181 & & \textbf{0.211} & 0.199 & 0.186 & & 0.235 & 0.219 & 0.202 \\
        TFT.multivar.comp.dist & & \textbf{0.201} & 0.187 & \textbf{0.177} & & 0.216 & \textbf{0.192} & \textbf{0.183} & & \textbf{0.232} & \textbf{0.210} & \textbf{0.196} \\
    \hline
    \end{tabular}
}
\caption{Model performance comparison of all model and clustering configurations in three forecasting horizons (14 days, 30 days and 60 days)}
\label{table_results}
\end{sidewaystable}
